# Supplementary material for: Certain and Approximately Certain Models for Statistical Learning
Source: arXiv:2402.17926 source file (2024-03-01)
Supplement: Supplementary file 1 [file Supplementary_Materials.tex]

\section{Supplementary Materials}
\subsection{Proof to Algorithm \ref{alg:ACM-linear_regression}}
Algorithm \ref{alg:ACM-linear_regression} can be splitted to three steps below.

\noindent
{\textbf{Step 1: Finding interval-formatted orthogonal basis} Based on the Gram-Schmidt process \cite{leon2013gram}, we find the first basis vector $\mathbf{b}_1 = \mathbf{z}_1$, and then the second basis vector $\mathbf{b}_2 = \mathbf{z}_2 - \text{proj}_{\mathbf{b_1}}(\mathbf{z_2})$, so on so forth till $\mathbf{b}_{d}$. The last basis vector $\mathbf{b}_d = \mathbf{z}_d - \text{proj}_{\mathbf{b_1}}(\mathbf{z_d}) - ... - \text{proj}_{\mathbf{b_{d-1}}}(\mathbf{z_d})$. Projecting one interval vector onto another interval vector is efficiently implemented through an existing interval arithmetic solution \cite{jaulin2001interval}. As a result, we find orthogonal basis ($\mathbf{b}_1, ..., \mathbf{b}_d$) where $\mathbf{b}_i = [b_{i1}, ..., b_{in}]^T$ is uncertain but bounded by
\[
b_{i1}^{min} \leq b_{i1} \leq b_{i1}^{max}, ..., b_{in}^{min} \leq b_{in} \leq b_{in}^{max}
\]

\noindent
{\textbf{Step 2: Projecting Label Vector onto Orthogonal Basis} 
We perform linear regression with orthogonal basis vectors, and get linear coefficients $\beta_1, ..., \beta_d$. Due to the orthogonality, linear regression is simply computing inner products between the label vector and each basis vector:
\[
\mathbf{\beta}^T = [\beta_1, \ldots, \beta_d] = \mathbf{y}^\intercal \cdot [\mathbf{b}_1, \ldots, \mathbf{b}_d]
\]
Here, $\beta_1, \ldots, \beta_{d}$ are interval values because basis vectors are interval vectors. Again, the inner product operations above can be efficiently implemented through the existing solution. Denote $\beta_d = [\beta_d^{min}, \beta_d^{max}]$ where $\beta_d^{min} \leq \beta_d \leq \beta_d^{max}$. So far, we have passed uncertainty from missing data to linear regression model by $\mathbf{\beta}$. However, the linear regression model $\mathbf{\beta}$ is with respect to the orthogonal basis instead of the original training data. Hence, we need to transform $\mathbf{\beta}$ to $\mathbf{w}$, which is the linear regression model with respect to the original training data $\mathbf{X}$. 

\noindent
{\textbf{Step 3: Determining the bounds for linear regression models} From Step 2, we get the optimal linear regression model $\mathbf{\beta}$ such that:

\[
\mathbf{y} = \beta_1 \cdot \mathbf{b}_1 + ... + \beta_d \cdot \mathbf{b}_d + \mathbf{r}
\]

where $\mathbf{r}$ is the minimal regression residue. Now, we replace $\mathbf{b}_1, ..., \mathbf{b}_d$ with $\mathbf{z}_1, ..., \mathbf{z}_d$ to get optimal model $\mathbf{w}$ with respect to $\mathbf{X}$:

\[
\mathbf{y} = w_1 \cdot \mathbf{z}_1 + \dots + w_d \cdot \mathbf{z}_d + \mathbf{r}
\]

In this step, we find the model parameters in the format of intervals. As a result, we get bounds for each model parameter: $w_1^{min} \leq w_1 \leq w_1^{max}, ..., w_d^{min} \leq w_d \leq w_d^{max}$. Finally, the Euclidean distance between two possible models is bounded by $e = \sqrt{\sum_{i=1}^{d} (w_i^\text{max} - w_i^\text{min})^2}$.
